# Supplementary material for: Graph Profiling for Vertex Cover: Targeted Reductions in a Branch and Reduce Solver
Source: arXiv:2003.06639 source file (2020-03-14)
Supplement: Supplementary file 1 [file appendix_tables.tex]

\cmt{Add tables for runtimes of the four types (blg, OCT, dimacs, pace)
sorted by min runtime. For blg, need to be selective or group by degree
spread range. Alternatively, provide a table for each 'quadrant'
}

% [Last modified: 2019 08 13 at 21:08:30 GMT]
